# Supplementary material for: Geometric Sample Reweighting for Monte Carlo Integration
Source: arXiv:1908.01809 source file (2019-08-05)
Supplement: Supplementary file 1 [file appendix.tex]

%-------------------------------------------------------------------------
%\section{Proof of Effective Sample Density Properties}
%\label{apdx:properties}
%In this appendix we provide proof of properties listed in Section \ref{sec:georeweight:PHED:effectivedensity}.
%
%Given a valid set of samples $X = \left \{ x_i | x_i \in \Omega, i = 1, \dots, N \right \}$, the probability (chance, not density) of sampling one existing sample point is $0$.
%That is, $x_i \neq x_j, \forall i \neq j$ holds.
%Thus, there are no duplicated samples, but samples can be arbitrarily close to each other: $\forall i \neq j, \exists \epsilon \in \mathbb{R}^+ \textup{ such that } 0 < \left | x_i - x_j \right | \leq \epsilon$.
%
%\textbf{Property 1.} $p_{\textup{eff}}(x) > 0, \forall x \in \Omega $ \\
%Since $\Omega$ is finite, the subset $V \subseteq \Omega$ is finite and $|\Omega|$ is constant.
%Thus $N|V|$ is always finite, i.e., can not reach $\infty$.
%Thus $p_{\textup{eff}}(x) = \frac{\left | \Omega \right |}{N \left | V(x) \right |} > 0$ holds.
%Given that there are no duplicated samples, the private hypervolume $V(x)$ for sample $x$ can be arbitrarily small but greater than $0$: $\forall x \in \Omega, V(x)>0$.
%Thus $p_{\textup{eff}}(x) = \frac{\left | \Omega \right |}{N \left | V(x) \right |} < \infty$ also holds.
%
%%\textbf{Property 2.} $p_{\textup{eff}}(x) = 0, \forall x \notin \Omega $ \\
%%With reference to Definition \ref{def:privolume}, we know that for $x \notin \Omega$, there is no definition of private hypervolume associated.
%%Therefore we can treat $\forall x \notin \Omega$ be $x \in \Omega^\mathsf{c}, \textup{ where } \Omega \cap \Omega^\mathsf{c} = \emptyset \textup{ and } \Omega \cup \Omega ^\mathsf{c} = \mathbb{R}^d.$
%%Since $\Omega$ is finite, $\lim \left | \Omega^\mathsf{c} \right | = \lim \left | \mathbb{R}^d - \Omega \right| = \infty - \left | \Omega \right | = \infty$.
%%Thus $\forall x \notin \Omega, p_{\textup{eff}}(x) = \frac{\left| \Omega \right|}{N \left | \Omega^\mathsf{c} \right |} = \frac{\left| \Omega \right|}{ N \times \infty} = 0$.
%
%\textbf{Property 2.} $E\left[ p_{\textup{eff}}(x) \right] = p(x) $ \\
%\begin{align*}
%	E\left[ p_{\textup{eff}}(x) \right] &= E\left[ \frac{\left | \Omega \right |}{N \left | V(x) \right | } \right] = \frac{\left | \Omega \right |}{N} E\left[ \frac{1}{V(x)}\right] \\
%										&= \frac{\left | \Omega \right |}{N} \frac{1}{\frac{\left | \Omega \right |}{N p(x)}} = p(x).
%\end{align*}
%
%\textbf{Property 3.} $E\left[ \int_{\Omega} p_{\textup{eff}}(x) \d x \right] = 1 $ \\
%Given the property above, it is trivial to show that: $E\left[ \int_{\Omega} p_{\textup{eff}}(x) \d x \right] = \int_{\Omega} p(x) \d x = 1$.

%-------------------------------------------------------------------------

%\section{Uniformly Distributed Random Samples}
%\label{apdx:unbiasedness}

%Given a set of \textbf{i}ndependent and \textbf{i}dentically \textbf{d}istributed \textbf{uniform} samples $X = \left\lbrace x_i | x_i \in \Omega, i = 1, \dots, N \right\rbrace$ generated for a Monte Carlo integration process, the estimator with \emph{geometric reweighting} (GR) is given as:
%\begin{equation}
%\hat{I}_{GR} = \sum_{i=1}^{N} w_{GR}(x_i) f(x_i)\text{, where }w_{GR}(x_i) = \frac{1}{N} \frac{1}{p_{\textup{eff}}(x_i)}.
%\end{equation}
%
%The effective sample density $p_{\textup{eff}}(x_i)$ is given as follows:
%\begin{equation}
%p_{\textup{eff}}(x_i) = C(x_i) \frac{\left| \Omega \right|}{N \left|V_i\right|},
%\end{equation}
%where $\left|V_i\right|$ denotes the private hypervolume of sample $x_i$, $\left|\Omega\right|$ denotes the total hypervolume of domain $\Omega$ and $N$ is the cardinality of set $X$.
%$C(x_i)$ is the correction coefficient for sample $x_i$ and is used to correct sample weight according to sample location.
%
%\subsection{Correction Coefficient}
%\label{apdx:unbiasedness:correctcoef}
%\paragraph{Boundary Order}Given a set of $N$ (with $N\geq3^D$) samples in $D$ dimensions, i.e., $\Omega = \left[0, 1\right)^D$, we define the \emph{boundary order} $b(x_i)$ of a sample as how many dimensions of $D$ is the private hypervolume associated with $x_i$ at the boundary of sample set $X$ and $b(x_i)\in\left[0, D\right]$.
%For instance, in a one dimensional sample set, the two bounrary points are of boundary order $1$, i.e., $b(x_i)=1$, and all other sample points in between are of boundary order $0$, i.e., $b(x_i)=0$.
%We can get the boundary order of a sample during voronoization.
%
%The cardinality of samples at order $d$ is defined as: $\{x_*^d\} = \textup{card} \\ \left\{ b(x_i)=d, \forall i \in \left[1, N\right]\right\}$.
%For such a sample set as mentioned above, the expected cardinality of samples of order $d$ is $E[ \{ x_*^d \} ] = K_d = \binom{D}{d} (\sqrt[D]{N}-2)^d 2^{D-d}$, where $K_d$ \text{ is the } $d$-th term in the bionomial expansion $N = (\sqrt[D]{N})^D = [$\underline{($\sqrt[D]{N}-2$)}$ + \underline{2}]^D$.
%
%Let $n = \sqrt[D]{N}$ and $b_i$ as a short note of $b(x_i)$, the correction coefficient is given as:
%\begin{equation}
%	C(x_i) = \left(\frac{3}{2}\right)^{b_i} \frac{N}{n+1}.
%\end{equation}
%
%\subsection{Proof of Unbiasedness}
%\label{apdx:unbiasedness:proof}
%First we need to show that $\int p_{\textup{eff}} = 1$, then we need to show $E\left[p_{\textup{eff}}\right] = p$.
%Let's start with $1$D case.
%Given an ordered list of samples that are uniformly distributed, it can be shown that:
%\begin{equation}
%	E\left[ x_{i+1} - x_{i}\right] = E\left[ x_{j+1} - x_{j}\right], \forall i \neq j; i, j = 0,\dots, N.
%\end{equation}
%$x_0$ and $x_{N+1}$ will corresponds to the two boundary points of the range $[0, 1]$ respectively, i.e., $x_0 = 0, x_{N+1} = 1$.
%With this, we can see that the range is divided into $N+1$ non-overlapping and concatenating segments and that they are expected to be of equal size.
%When analysing sample positions of an ordered sample list, we can see that the expected position of the $i$-th sample is:
%\begin{equation*}
%	E\left[x_i\right] = \frac{i}{N + 1},
%\end{equation*}
%thus the expected private hypervolume will be:
%\begin{equation*}
%	E\left[ V_i\right]=
%	\left\{
%	\begin{array}{lr}
%	\frac{3}{2} \frac{1}{N+1},& i = 1 \text{ or } N;\\
%	\frac{1}{N+1},& i \neq 1, i \neq N.
%	\end{array}\right.
%\end{equation*}
%Therefore, we have:
%\begin{align*}
%	\int p_{\textup{eff}} &= \frac{1}{N} \left(2^1 \times \frac{3}{2}\frac{N}{N+1} \frac{1}{N\frac{3}{2}\frac{N}{N+1}} + (N-2)\frac{N}{N+1} \frac{1}{N\frac{1}{N+1}}\right) \\
%	&= \frac{1}{N} \left( 2 + N - 2 \right) = 1
%\end{align*}
%
%Plugging everything together, we have:
%\begin{align*}
%	E\left[p_{\textup{eff}}\right] &= E\left[ C(x_i) \frac{\left| \Omega \right|}{N \left|V_i\right|} \right] = \frac{\left|\Omega\right|}{N}  E\left[ \frac{C(x_i)}{\left|V_i\right|} \right] \\
%	&= \frac{\left|\Omega\right|}{N} \left\{ \frac{1}{N} \left( \frac{3}{2} \frac{N}{N+1} \frac{1}{\frac{3}{2} \frac{1}{N+1}} \times 2 + \frac{N}{N+1} \frac{1}{\frac{1}{N+1}} \times (N-2))\right) \right\} \\
%	&= \left|\Omega\right| = 1 = p(x_i).
%\end{align*}
%
%To generalize this into $D$ dimensions, consider the following:
%given a meaningful metric, e.g., grid hierarchy, such that we can locate samples in hyper space $\Omega$.
%For $D$ dimensions, we have samples of $D+1$ orders of boundary, i.e., $0, \dots, N$.
%Since we are dealing with i.i.d., uniform distribution, we have for each dimension expected $n +1 = \sqrt[D]{N} + 1$ resolutions.
%Then we have:
%\begin{align*}
%	E\left[V_i\right] &= \left(\frac{3}{2}\right)^{b_i}\frac{1}{n+1}
%\end{align*}
%
%Plug in, we have:
%\begin{align*}
%	\int p_{\textup{eff}} &= \frac{1}{N} E\left[\frac{\left|\Omega\right|C(x_i^d)}{N\left|V_i\right|} \right] = \frac{\left|\Omega\right|}{N} \sum |x_i^d| \frac{C(x_i^d)}{N\times E\left[\left|V_i\right|\right]} \\
%	&= \frac{\left|\Omega\right|}{N} \sum \binom{D}{d} (n-2)^d 2^{D-d} \left(\frac{3}{2}\right)^d \frac{N}{n+1} \frac{1}{N\times E\left[V_i\right]} \\
%	&= \frac{\left|\Omega\right|}{N} N = \left|\Omega\right| = 1.
%\end{align*}
%
%Therefore, we have:
%\begin{align*}
%E\left[p_{\textup{eff}}(x_i)\right] &= E\left[ C(x_i) \frac{\left| \Omega \right|}{N \left|V_i\right|} \right] = \frac{\left|\Omega\right|}{N}  E\left[ \frac{C(x_i)}{\left|V_i\right|} \right] \\
%	&= \frac{\left|\Omega\right|}{N} \left(\frac{3}{2}\right)^d \frac{N}{n+1} \times \frac{1}{E\left[V_i\right]} \\
%	&= \frac{\left|\Omega\right|}{N}\times N =\left|\Omega\right| =1 = p(x_i).
%\end{align*}
%Therefore $E\left[ \hat{I}_{GR} \right] = I$.
%
%\subsection{Case with Stratified Sample Set}
%For samples generated with stratification, we can treat each stratum as an independent unit and the whole range as a composition of such units.
%Then for a sample set $X$ of size $N$ generated with $S$ strata, each stratum is expected to share $\frac{N}{S}$ samples.
%Let $n = \sqrt[D]{N}$ and $s = \sqrt[D]{S}$, we can further generalize the correction coefficient to:
%\begin{equation}
%C(x_i) = \left(\frac{3}{2}\right)^{b_i} \frac{N}{n+s}.
%\end{equation}
%
%Given the proof above that for a single range, $E[\hat{I}_{\Omega, GR}]=I_\Omega$, we can see that this relation holds for each stratum, i.e., $E[\hat{I}_{st, GR}] = E\left[\hat{I}_{st}\right] = I_{st}$.
%Considering the fact that the MC estimator with stratification $\hat{I}^{s}_\Omega$ is the average of all small stratum estimators, the following holds as well:
%\begin{align*}
%	E\left[\hat{I}^{s}_{\Omega, GR}\right] &= \frac{1}{S} E\left[ \sum_{j=1}^{S} \hat{I}_{j, GR}^s \right] = \frac{1}{S} \sum_{j=1}^{S} E\left[ \hat{I}_{j, GR}^s \right] \\
%	&= \frac{1}{S} \sum_{j=1}^{S} E\left[ \hat{I}_{j}^s \right] = E\left[ \hat{I} \right] = I.
%\end{align*}
%Therefore, for MC estimator with stratification, $E\left[ \hat{I}_{GR} \right] = I$ holds.
%
%
%\section{Generalised Geometric Sample Reweighting}
%With the proof above, we provide the generalized geometric sample reweighting for a set of $N$ $D$-dimensional samples generated with $S$ strata for domain $\Omega\subseteq[0, 1)^D$ as follows:
%\begin{align*}
%\hat{I}_{GR} &= \sum_{i=1}^{N} w_{GR}(x_i) f(x_i), \\
%w_{GR}(x_i) &= \frac{1}{N} \frac{1}{p_{\textup{eff}}(x_i)}, \\
%p_{\textup{eff}}(x_i) &= C(x_i) \frac{\left| \Omega \right|}{N \left|V_i\right|}, \\
%C(x_i) &= \left(\frac{3}{2}\right)^{b_i} \frac{N}{n+s}, n = \sqrt[D]{N}, s = \sqrt[D]{S}, \\
%b_i &= b(x_i)\text{, the boundary order of sample }x_i.
%\end{align*}
%

%%-------------------------------------------------------------------------
%\section{Unbiasedness and Working in Batches}
%\label{apdx:D}
%\paragraph{Unbiasedness}
%Incorporating Equation \ref{eq:importance:volumescaling}, \ref{eq:weightedRSum}, \ref{eq:effdensitydefinition} and \ref{eq:MCGeoRW}, our MC estimator with geometric reweighting is essentially:
%\begin{equation*}
%	\hat{I}_{GR} = \frac{1}{N} \sum_{i=1}^{N} \frac{f(x_i)}{p_{\textup{eff}}(x_i)}.
%\end{equation*}
%Thus, given \textbf{Property 3} above, we have:
%\begin{align*}
%E\left[\hat{I}_{GR}\right] 	&= E\left[\frac{1}{N} \sum_{i=1}^{N} \frac{f(x_i)}{p_{\textup{eff}}(x_i)}\right] = \frac{1}{N} \sum_{i=1}^{N} E\left[\frac{f(x_i)}{p_{\textup{eff}}(x_i)}\right] \\
%							&= \frac{1}{N} \sum_{i=1}^{N} E\left[\frac{f(x_i)}{p(x_i)}\right] = \int_{\Omega} f(x) \d x = I.
%\end{align*}
%
%\paragraph{Working in Batches}
%As one of nice features of the original MC integrators, provided that all samples are following independent and identical distribution (i.i.d), results from different batches can be combined in whichever way one would like to and still remain unbiased.
%
%The MC integrator can be conveniently decomposed into $k$ independent batches:
%\begin{equation*}
%	\hat{I} = \frac{1}{N} \sum_{i=1}^{N} \frac{f(x_i)}{p(x_i)} = \sum_{i=1}^{k} w(k) \frac{1}{N_k} \sum_{j=1}^{N_k} \frac{f(x_j)}{p(x_j)},
%\end{equation*}
%where $w(k) = \frac{N_k}{N}$ and $\sum N_k = N$.
%
%For MC integrator with geometric reweighting, by adding multiple batches together, we have the following:
%\begin{equation*}
%	\hat{I}_{GR}^{\textup{batch}} = \frac{N_1}{N} \hat{I}_{GR}^{N_1} + \frac{N_2}{N} \hat{I}_{GR}^{N_2} + \dots + \frac{N_k}{N} \hat{I}_{GR}^{N_k},
%\end{equation*}
%where $\sum N_i = N$.
%The expectation of this estimator is:
%\begin{align*}
%	E\left [ \hat{I}_{GR}^{\textup{batch}}  \right ] 	&= E\left [ \frac{N_1}{N} \hat{I}_{GR}^{N_1} + \frac{N_2}{N} \hat{I}_{GR}^{N_2} + \dots + \frac{N_k}{N} \hat{I}_{GR}^{N_k}  \right ] \\
%														&= E\left [\frac{N_1}{N} \hat{I}_{GR}^{N_1} \right ] + E\left [ \frac{N_2}{N} \hat{I}_{GR}^{N_2}\right ] + \dots + E\left [ \frac{N_k}{N} \hat{I}_{GR}^{N_k} \right ] \\
%														&= \frac{N_1}{N} E\left [ \hat{I}_{GR}^{N_1}\right ] + \frac{N_2}{N} E\left [ \hat{I}_{GR}^{N_2}\right ] + \dots + \frac{N_k}{N} E\left [ \hat{I}_{GR}^{N_k}\right ] \\
%														&= \frac{N_1}{N} I + \frac{N_2}{N} I + \dots + \frac{N_k}{N} I = I.\\
%\end{align*}
%
%In summary, MC integration with geometric sample reweighting is unbiased and can work in batches.

% ============================================================================
% End of appendix.tex 
